# Supplementary material for: Divide&Classify: Fine-Grained Classification for City-Wide Visual Place Recognition
Source: arXiv:2307.08417 source file (2023-12-06)
Supplement: Supplementary file 1 [file supp_ablation_backbones.tex]

\begin{table}
\centering
\begin{adjustbox}{width=0.75\linewidth}
\begin{tabular}{lcccc}
\toprule
\multirow{2}{*}{Backbone} & 
\multicolumn{4}{c}{Great Circle Distance (GCD)} \\
\cline{2-5}
\multicolumn{1}{c}{}
& 25m & 50m & 100m & 500m \\
\hline
ResNet-50 \cite{He_2016_resnet}              & 52.0 & 54.7 & 55.6 & 59.0 \\
EfficientNet-B0 \cite{Tan_2019_efficientnet} & 49.2 & 52.8 & 53.5 & 57.8 \\
EfficientNet-B4 \cite{Tan_2019_efficientnet} & 54.3 & 57.1 & 57.6 & 61.5 \\
EfficientNet-B5 \cite{Tan_2019_efficientnet} & 56.9 & 60.0 & 60.1 & 63.3 \\
EfficientNet-B7 \cite{Tan_2019_efficientnet} & 62.1 & 64.9 & 65.4 & 67.6 \\
ViT \cite{Dosovitskiy_2021_vit}             & 48.9 & 51.5 & 52.2 & 57.1 \\
CCT \cite{Hassani_2021_cct}                 & 39.8 & 43.8 & 45.9 & 50.4 \\
\bottomrule
\end{tabular}
\end{adjustbox}
\caption{\textbf{Ablation on various backbones} on SF-XL.}
\label{tab:supp_ablation_backbones}
\end{table}
