# Supplementary material for: Divide&Classify: Fine-Grained Classification for City-Wide Visual Place Recognition
Source: arXiv:2307.08417 source file (2023-12-06)
Supplement: Supplementary file 2 [file supp_cplanet_distances.tex]

\begin{table}
\begin{adjustbox}{width=\linewidth}
\centering
\begin{tabular}{l|cccc}
\toprule
 & SF-XL & C-Pitts30k & C-Pitts250k & C-Tokyo 24/7 \\
\hline
HGE-coarse & 23.41 & 20.27 & 21.09 & 42.00\\
HGE-medium & 14.37 & 13.16 & 12.26 & 24.86\\
HGE-fine   &  8.67 & 6.81 & 6.91 & 16.78\\
CPlaNet &  10.17 &  9.74 &   9.75 & 10.89 \\
\bottomrule
\end{tabular}
\end{adjustbox}
\caption{\textbf{Mean of distances between each image and the center of its class} \gb{TODO}}
\label{tab:supp_cplanet_distances}
\end{table}
